# Supplementary material for: Offsite-Tuning: Transfer Learning without Full Model
Source: arXiv:2302.04870 source file (2023-02-09)
Supplement: Supplementary file 1 [file a_appendix.tex]

\newpage
\appendix
\onecolumn
\section{You \emph{can} have an appendix here.}

You can have as much text here as you want. The main body must be at most $8$ pages long.
For the final version, one more page can be added.
If you want, you can use an appendix like this one, even using the one-column format.
